# Supplementary material for: SpectralCanary: Embarrassingly Simple Low-Frequency Traces for T2I Dataset-Use Auditing
Source: arXiv:2610.31659 source file (2026-10-22)
Supplement: Supplementary file 2 [file detailed_data_construction.tex]

\section{Supplementary Material for Data Construction}
\label{sec:supp:data-construction}

\subsection{Prompt to Extract Proposal}\label{sec:supp:prompt-extract}\label{Sec: Prompt to Extract Proposal}

The prompt is designed to extract proposal-level content from each paper while explicitly excluding results and conclusions. The proposal format follows \cite{yamada2025aiscientistv2}.

\begin{tcolorbox}[title=\textbf{System Prompt to Extract Proposal}]
\small

You are an expert at extracting structured research information from machine learning papers. Extract the research proposal in \textit{AI Scientist v2} format, capturing the intended hypothesis and experimental design \textbf{before any experimental results}. The goal is to represent the research plan and claims prior to execution, not confirmed findings.

\textbf{Output:} Return \textbf{valid JSON only}. Do not include markdown or explanations.

\vspace{0.3em}
\textbf{Global Principles}
\begin{itemize}
\item Extract only proposal-level content; exclude results and conclusions.
\item Prefer verbatim spans from the paper when possible.
\item Do not hallucinate or introduce structure not present in the paper.
\item If uncertain, omit the information.
\item Keep claims atomic and directly grounded in the source text.
\end{itemize}

\vspace{0.3em}
\textbf{Hypothesis}
\begin{itemize}
\item Extract from Introduction or Method sections.
\item Describe what the paper proposes or aims to test (1--2 sentences).
\item Prefer verbatim phrasing.
\end{itemize}

\textbf{Forbidden:} ``we show'', ``we demonstrate'', ``we find'', ``results show'', ``outperforms'' \\
\textbf{Allowed:} ``we propose'', ``we hypothesize'', ``we argue'', ``our approach aims to''

\vspace{0.3em}
\textbf{Experiments}
\begin{itemize}
\item Describe experimental plan only (no results or numbers).
\item Each entry must correspond to a distinct experiment group.
\end{itemize}

\textbf{Description:} goal of the experiment. \\
\textbf{Method:} datasets, models, baselines, setup (preserve exact names). \\
\textbf{Metrics:} list evaluation metrics (no values).

\vspace{0.3em}
\textbf{Related Work}
\begin{itemize}
\item Summarize prior work and research gap.
\item Do not include improvement claims.
\end{itemize}

\vspace{0.3em}
\textbf{Risk Factors}
\begin{itemize}
\item Extract explicit limitations from the paper.
\item Do not infer or invent new risks.
\end{itemize}

\vspace{0.3em}
\textbf{Abstract}
\begin{itemize}
\item Keep only problem, motivation, and proposed method.
\item Remove results, numbers, and comparisons.
\end{itemize}

\end{tcolorbox}

\begin{tcolorbox}[title=\textbf{User Prompt to Extract Proposal}]
\small

\textbf{Input}
\begin{itemize}
\item \textbf{Abstract:}
\begin{verbatim}
{abstract}
\end{verbatim}
\item The attached file is the \textbf{full paper PDF}.
\end{itemize}

Use both the abstract and the PDF to extract the research idea.

\vspace{0.3em}
\textbf{Instructions}
\begin{itemize}
\item Extract the \textbf{Short Hypothesis} from the \textbf{Introduction or Method sections}, not from results or conclusions.
\item All \textbf{Experiment fields} must reflect the \textbf{experimental plan}, not observed outcomes.
\item Preserve \textbf{dataset names, tasks, and baselines} when describing experiments.
\item Create \textbf{multiple experiment entries} if the paper evaluates multiple tasks or benchmarks.
\end{itemize}

\vspace{0.3em}
\textbf{Output Format (JSON)}
\begin{verbatim}
{
  "Name": "<short slug identifying the research contribution>",
  "Title": "<exact paper title>",
  "Short Hypothesis": "<proposed claim or method — no outcomes>",
  "Related Work": "<prior work and research gap>",
  "Abstract": "<problem + motivation + proposed method only>",
  "Experiments": [
    {
      "Description": "<goal of this experiment group>",
      "Method": "<datasets/tasks, model setup, baselines>",
      "Evaluation Metrics": "<metrics used>"
    }
  ],
  "Risk Factors and Limitations": [
    "<explicit limitation sentence from the paper>"
  ]
}
\end{verbatim}

\vspace{0.3em}
\textbf{Critical Constraints}
\begin{itemize}
\item Do \textbf{not} include results or conclusions.
\item Do \textbf{not} include numerical values or measured performance.
\item Do \textbf{not} reveal whether the hypothesis was confirmed.
\item Do \textbf{not} generalize dataset names.
\item Do \textbf{not} merge distinct experiments into a single entry.
\end{itemize}

\end{tcolorbox}

\subsection{Prompt to Decompose Atomic Claims from Proposal}\label{sec:supp:prompt-decompose}\label{Sec: Prompt to Decompose Atomic Claims from Proposal}

This prompt decomposes each proposal into minimal, independently verifiable factual claims so that each statement can be assessed clearly and grounded in source text. The detailed process is presented in Alg.~\ref{alg:verification}. We compute extraction faithfulness with a retrieval-backed atomic-claim score by decomposing each hypothesis--experiment pair into atomic claims, retrieving supporting passages, and verifying each claim against the source paper, following prior work on atomic factuality and evidence-grounded verification~\citep{min-etal-2023-factscore,thorne2018fever}. We use GPT-5.4 for this process.




\begin{tcolorbox}[title=\textbf{System Prompt to Decompose Atomic Claims from Proposal}]
\small

You are a precise scientific analyst. Your task is to decompose a research hypothesis and experimental plan into atomic, independently verifiable claims.

\end{tcolorbox}

\vspace{1.0cm}

\begin{tcolorbox}[title=\textbf{User Prompt to Decompose Atomic Claims from Proposal}]
\small

\textbf{Task.} Decompose the following extraction into \textbf{atomic factual claims} that are directly verifiable from the paper text.

\vspace{0.3em}
\textbf{Rules}
\begin{itemize}
\item Output \textbf{one complete claim per line}.
\item Do not include numbering, bullets, prefixes, section headers, or commentary.
\item Do not output incomplete fragments.
\item Do not introduce synthetic labels (e.g., ``Experiment 1'', ``Experiment 2'').
\item Keep claims literal and close to wording likely present in the paper.
\end{itemize}

\vspace{0.3em}
\textbf{Scope of Claims}
Include only claims about:
\begin{itemize}
\item proposed method or hypothesis
\item planned evaluation setup
\item datasets, tasks, and baselines
\item evaluation metrics
\end{itemize}

Exclude:
\begin{itemize}
\item any result or outcome claims (e.g., ``improves'', ``outperforms'', ``achieves state-of-the-art'')
\end{itemize}

\vspace{0.3em}
\textbf{Input Extraction}
\begin{verbatim}
{extraction_proposal}
\end{verbatim}

\end{tcolorbox}

\subsection{Prompt to Verify Atomic Claims}\label{sec:supp:prompt-verify}

This prompt evaluates each claim--evidence pair and produces a concise YES/NO judgment so that verification decisions remain explicit, consistent, and grounded in the provided textual evidence. We use Gemini-2.5-Flash for this process.

\vspace{1.0cm}

\begin{tcolorbox}[title=\textbf{System Prompt to Verify Atomic Claims}]
\small

You are a rigorous scientific fact-checker. Your task is to verify whether a claim is \textbf{directly supported} by the provided evidence from a paper.

\end{tcolorbox}

\begin{tcolorbox}[title=\textbf{User Prompt for Atomic Claim Verification}]
\small

\textbf{Input Claim}
\begin{verbatim}
{claim}
\end{verbatim}

\textbf{Evidence (excerpts from the paper)}
\begin{verbatim}
{evidence}
\end{verbatim}

\vspace{0.3em}
\textbf{Task}

Determine whether the claim is \textbf{directly supported} by the provided evidence.

\vspace{0.3em}
\textbf{Output Format}

Reply with exactly:
\begin{verbatim}
YES/NO: <one-sentence explanation>
\end{verbatim}

\end{tcolorbox}

\subsection{\fh{Preliminary Human Audit of Extraction Quality and Label Validity}}
\label{sec:supp:human-audit}

\tuyen{To complement the automated retrieval-backed audit, we conduct a preliminary human verification audit focused on the concerns that are hardest to resolve automatically: explicit result leakage, outcome-revealing language, acceptance clues, and whether the assigned reviewer-derived soundness label is defensible from the extracted proposal alone. Annotators are not shown the full original paper. They see only the extracted experiment plan and benchmark label to audit. The audit is designed as a quality-control check rather than as a full expert-ceiling study. In particular, reviewers of the original papers saw full manuscripts and results, whereas evaluated models and audit annotators see results-masked proposal text. Therefore, the goal of this audit is to test whether the constructed examples are broadly usable as proposal-stage proxies, not to claim perfect equivalence with full-paper peer review or to estimate the maximum possible human performance on the task.}

\tuyen{Two annotators independently inspect a balanced subset of low- and high-soundness proposals using this proposal-only view. For each proposal, annotators answer three binary questions: (1) whether the extracted proposal leaks numerical results or direct outcome claims; (2) whether it contains acceptance clues or post-hoc framing; and (3) whether the assigned soundness label is supported by the proposal content alone. We treat disagreement and unsupported-label cases as diagnostic signals for future filtering rather than resolving them away. In the currently completed audited subset, 92.3\% of leakage checks match the expected ``No'' answer, and 84.6\% of label-validity checks match the expected ``Yes'' answer. These preliminary results suggest that the extraction pipeline usually avoids explicit outcome leakage and that reviewer-derived soundness labels are broadly defensible as a practical proxy, while also confirming that proposal-only soundness remains an imperfect and intrinsically limited target. We report this small 60-proposal audit separately and use it to guide larger-scale expert re-annotation in future versions.}

\begin{table}[h]
\centering
\caption{\fh{Preliminary human audit results for extraction quality and label validity.}}
\label{tab:human_audit}
\begin{tabular}{lc}
\toprule
\fh{\textbf{Audit question}} & \fh{\textbf{Agreement rate}} \\
\midrule
\fh{Leakage of numerical results or direct outcome claims?} & \fh{92.3\% expected No} \\
\fh{Assigned soundness label is defensible?} & \fh{84.6\% expected Yes} \\
\bottomrule
\end{tabular}
\end{table}

\subsection{Example of Extracted Proposals}\label{sec:supp:proposal-examples}

We provide two extracted-proposal examples from SoundnessBench: one high-soundness case and one low-soundness case. The benchmark contains 458 low-soundness and 641 high-soundness instances in total. The format of these proposals follows \citep{yamada2025aiscientistv2}.

\begin{tcolorbox}[title=\textbf{Example: High-Soundness Proposal}]
\small
\raggedright

\textbf{Paper id}: FUaDMRVrbS \\

\textbf{Identifiability for Gaussian Processes with Holomorphic Kernels} \\

\textbf{Year}: 2025 \\

\textbf{Short Hypothesis} \\
A novel theoretical framework, based on the property of kernels being holomorphic around zero, can determine the identifiability of parameters in a wide range of GP kernels (e.g., squared exponential, periodic, rational quadratic) and their complex combinations, filling a gap left by methods that only apply to Matérn-type kernels. \\

\textbf{Related Work} \\
\textit{[Content omitted for brevity]} \\

\textbf{Abstract} \\
\textit{[Content omitted for brevity]} \\

\textbf{Experiments}

\textit{Experiment 1} \\
\textbf{Description:} To empirically support the theoretical results on parameter identifiability for several individual holomorphic kernels. \\
\textbf{Method:} The experiment involves estimating parameters for individual Squared Exponential (SE), Damped Periodic (DPer), Periodic (Per), Rational Quadratic (RQ), and Cosine kernels. This is done by fitting a GP model to synthetically generated data of increasing sample sizes ($n \in \{500, 1000, 2000, 5000\}$) with added Gaussian noise. The parameters are estimated using Maximum Likelihood Estimators (MLEs). \\
\textbf{Evaluation Metrics:} Convergence of the Maximum Likelihood Estimators (MLEs) for each parameter over 100 replicates.

\vspace{0.5em}
\textit{Experiment 2} \\
\textbf{Description:} To empirically support the theoretical results on parameter identifiability for a complex combined kernel, specifically the one from Equation (2) motivated by the Mauna Loa CO2 dataset. \\
\textbf{Method:} A GP with the combined kernel from Equation (2) is fitted to synthetically generated data designed to mimic the properties of the Mauna Loa dataset over a 45-year time interval. The experiment uses increasing sample sizes ($n \in \{50, 100, 200, 500\}$), and the Maximum Likelihood Estimators (MLEs) for the kernel's 10 parameters are computed. \\
\textbf{Evaluation Metrics:} Convergence of the Maximum Likelihood Estimators (MLEs) for each parameter in the combined kernel over 100 replicates. \\


\textbf{Risk Factors and Limitations}
\begin{itemize}
\item First, while establishing the identifiability of kernel parameters is a critical step, it does not necessarily guarantee the consistency of the MLE.
\item Second, extending our theoretical framework to encompass non-stationary kernels ... remains a largely open problem.
\item Third, another intriguing direction involves extending findings to infinitely differentiable kernels not holomorphic near 0.
\end{itemize}

\vspace{0.3em}
\textbf{Scores:}
\begin{itemize}
  \item Soundness: 3.25
  \item Support Ratio: 1.0
  \item Rigor Bucket: high
\end{itemize}

\end{tcolorbox}


\begin{tcolorbox}[title=\textbf{Example: Low-Soundness Proposal}]
\small
\raggedright

\textbf{Paper id}: h9ThYkkgSD4 \\

\textbf{Activation Function: Absolute Function,One Function Behaves more Individualized} \\

\textbf{Year:} 2023 \\

\textbf{Short Hypothesis} \\
Using the absolute value function, y=|x|, as a neural network activation will result in more \"individualized\" representations by preserving information from negative inputs, unlike ReLU. This property is hypothesized to make it more suitable for generation tasks and potentially less prone to overfitting compared to ReLU and Leaky ReLU.\\

\textbf{Related Work} \\
\textit{[Content omitted for brevity]} \\

\textbf{Abstract} \\
\textit{[Content omitted for brevity]} \\

\textbf{Experiments}

\textit{Experiment 1} \\
\textbf{Description:} To evaluate the performance of the absolute activation function against standard activations in a fully-connected neural network on an image classification task.\\
\textbf{Method:} A 5-layer fully-connected neural network will be trained on the MNIST dataset. The performance of the absolute function will be compared against ReLU and Leaky ReLU as baselines. The experiment will use the Adam optimizer and SparseCategoricalCrossentropy loss. The effect of different batch sizes will also be investigated. \\
\textbf{Evaluation Metrics:} ['Training Accuracy', 'Validation Accuracy', 'Training Loss', 'Validation Loss']

\vspace{0.5em}
\textit{Experiment 2} \\
\textbf{Description:} To evaluate the performance of the absolute activation function in a convolutional neural network (CNN) on an image classification task and to visualize the resulting feature maps. \\
\textbf{Method:} A CNN with 3 convolutional layers and 2 fully-connected layers will be trained on the MNIST dataset. The absolute function will be compared against ReLU and Leaky ReLU baselines. The experiment will explore the effect of varying batch sizes (32, 64, 128). Additionally, the intermediate activations from the convolutional layers will be visualized for both the absolute function and ReLU to qualitatively compare the learned features. \\
\textbf{Evaluation Metrics:} ['Training Accuracy', 'Validation Accuracy', 'Training Loss', 'Validation Loss', 'Qualitative visualization of intermediate activations'] 

\vspace{0.5em}
\textit{Experiment 3} \\
\textbf{Description:} To test the hypothesis that the \"individualization\" property of the absolute function makes it well-suited for image generation tasks using an autoencoder. \\
\textbf{Method:} A functionally separate autoencoder, with a convolutional encoder and a corresponding decoder, will be trained on the MNIST dataset. The experiment will compare the image generation quality when using the absolute function in the encoder versus using a Leaky ReLU baseline. The model will use the Adam optimizer and MSE loss. \\
\textbf{Evaluation Metrics:} ['Qualitative comparison of generated output images'] \\

\textbf{Risk Factors and Limitations}
\begin{itemize}
\item In order to generalization, the individualization is the reason of shake, the accuracy may be good in some set and may be worse in some set.
\end{itemize} 

\textbf{Scores:}
\begin{itemize}
  \item Soundness: 1.0
  \item Support Ratio: 1.0
  \item Rigor Bucket: low
\end{itemize}

\end{tcolorbox}

\subsection{Example of Extracted Atomic Claims and Verification}\label{sec:supp:atomic-example}


\begin{tcolorbox}[title=\textbf{Example: Atomic Claims from Extracted Proposal}]
\small

\textbf{Source:} Identifiability for Gaussian Processes with Holomorphic Kernels

\vspace{0.3em}
\textbf{Atomic Claims (excerpt)}

\begin{itemize}
\item A novel theoretical framework is based on kernels being holomorphic around zero.
\item The framework determines identifiability of parameters in a wide class of Gaussian Process kernels.
\item The framework applies to squared exponential, periodic, and rational quadratic kernels.
\item The framework applies to complex combinations of kernels.
\item The framework addresses a gap left by methods that only apply to Matérn-type kernels.
\item A Gaussian Process model is fitted to synthetically generated data with added Gaussian noise.
\item Parameters are estimated using Maximum Likelihood Estimators.
\item Experiments evaluate convergence of estimators as sample size increases.
\end{itemize}

\vspace{0.3em}
\textbf{Summary:} 17 atomic claims extracted; all verified as supported (support ratio = 1.0).

\end{tcolorbox}
